# Supplementary material for: On the Optimization of Multi-Cloud Virtualized Radio Access Networks
Source: arXiv:2002.10681 source file (2020-02-26)
Supplement: Supplementary file 1 [file Appendix2.tex]

\section{Supplementary Material} \label{sec:appendix}
More...
